# Supplementary material for: Search for proton decay into three charged leptons in 0.37 megaton-years exposure of the Super-Kamiokande
Source: arXiv:2001.08011 ancillary file (2020-01-23)
Supplement: Supplementary file 1 [file supplemental_material_v20200116.pdf]

# Observed candidates



**Notes for candidates**
**(p→$e^+\mu^+\mu^-$ and p→$\mu^+\mu^+\mu^-$ modes)**

- Some of lower visible energy rings close to the higher visible energy rings are discarded by the final stage of ring counting.
  (Event displays in p2, 3)

# Observed candidate ($p \to e^+ \mu^+ \mu^-$ & $p \to e^- \mu^+ \mu^+$)



- SK4 (October 31st, 2012), run # 70589, sub run # 180, event # 37485314
- Total mass = 882.4 MeV/$c^2$, Total momentum = 159.8 MeV/c
- Distance between vertex and nearest wall = 608.6 cm
- Vertex X/Y/Z = -400.1 / 1004.7 / -54.5 cm

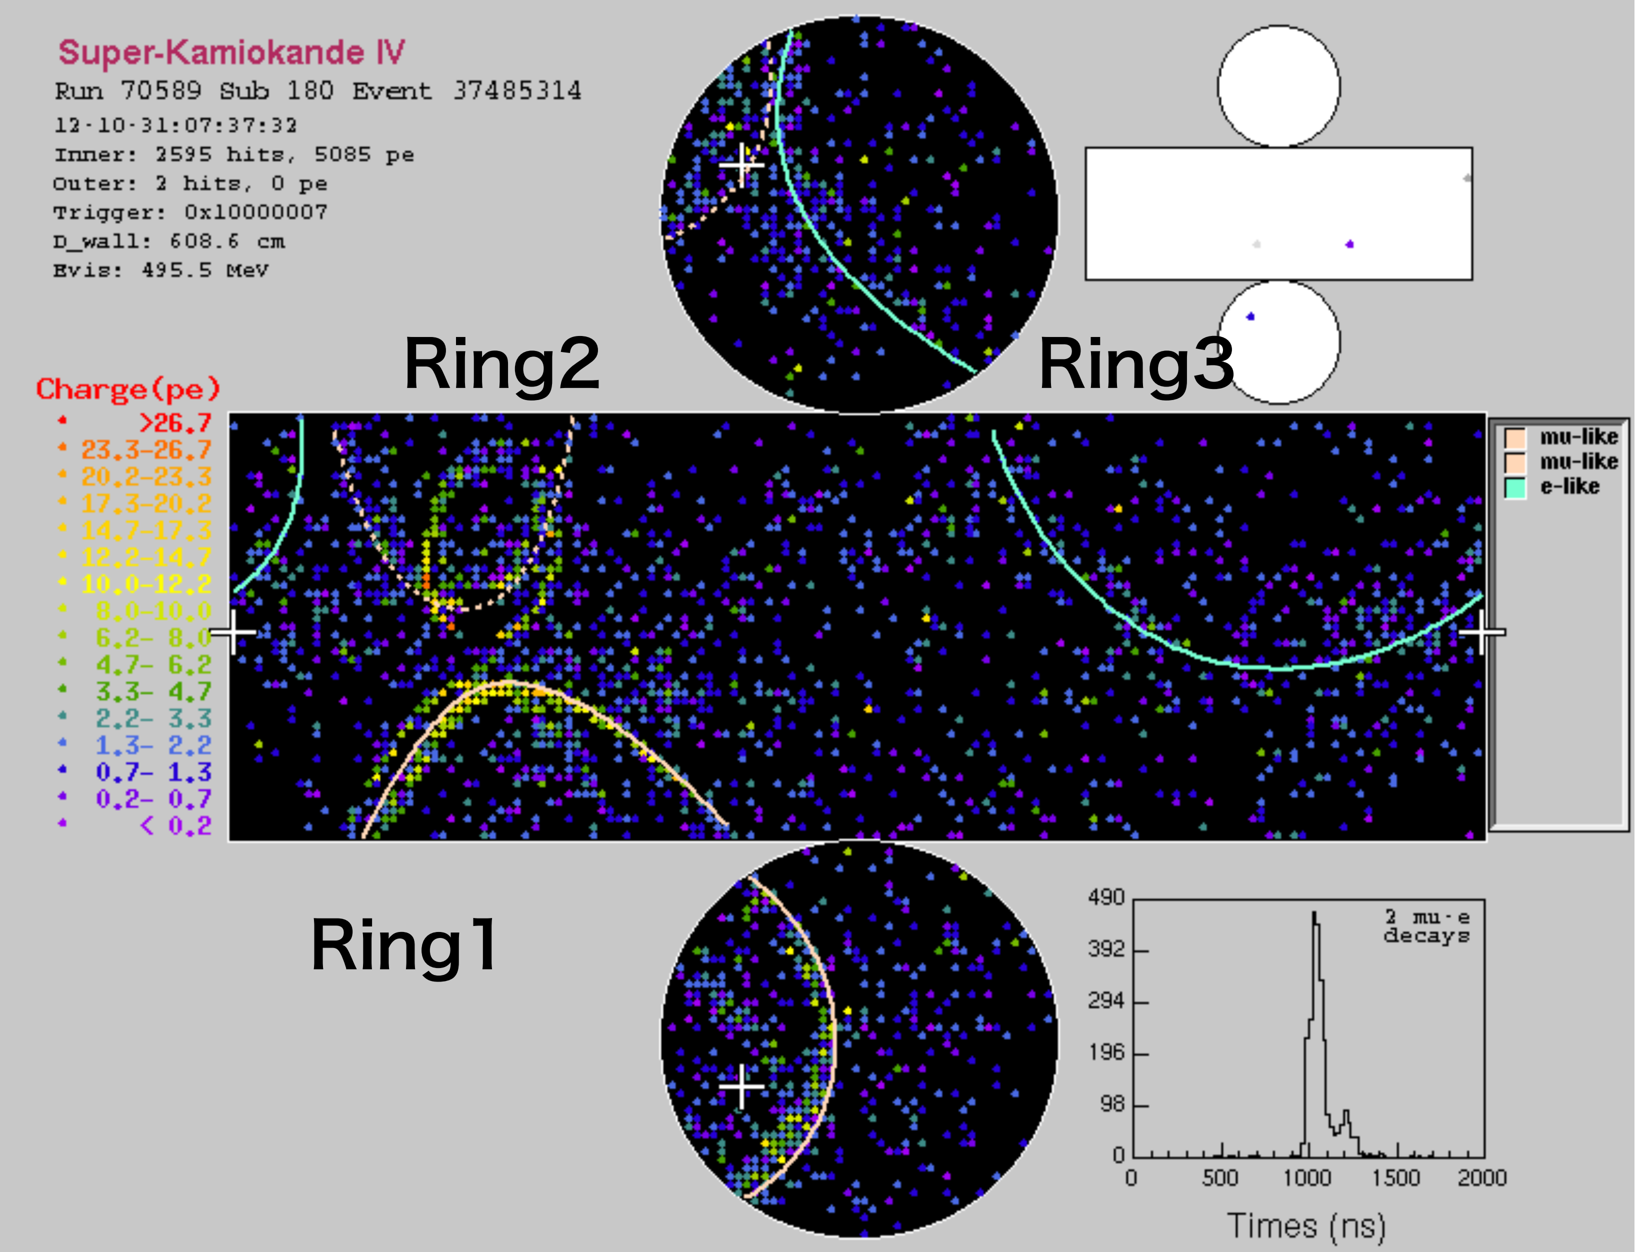


**Ring1**

PID: 0.82 → $\mu$-like

Opening angle → 40.3 deg.

Momentum → 412.3 MeV/c

(expected opening angle → 39.2 deg.)

**Ring2**

PID: 1.87→ $\mu$-like

Opening angle → 33.8 deg.

Momentum → 296.7 MeV/c

(expected opening angle → 37.2 deg.)

**Ring3**

PID: -3.4→ e-like

Opening angle → 43.1 deg.

Momentum → 156.2 MeV/c

(expected opening angle → 41.4 deg.)

# Observed candidate (p→$\mu^+\mu^+\mu^-$)



- SK1(June 11th, 2000), run # 8854, sub run # 245, event # 36673156
- #Decay-e = 2, Total mass = 835.1 MeV/c$^2$, Total momentum = 170.0 MeV/c
- Distance between vertex and nearest wall = 516.3 cm
- Vertex X/Y/Z = -357.3 / 1118.0 / -1270.3 cm

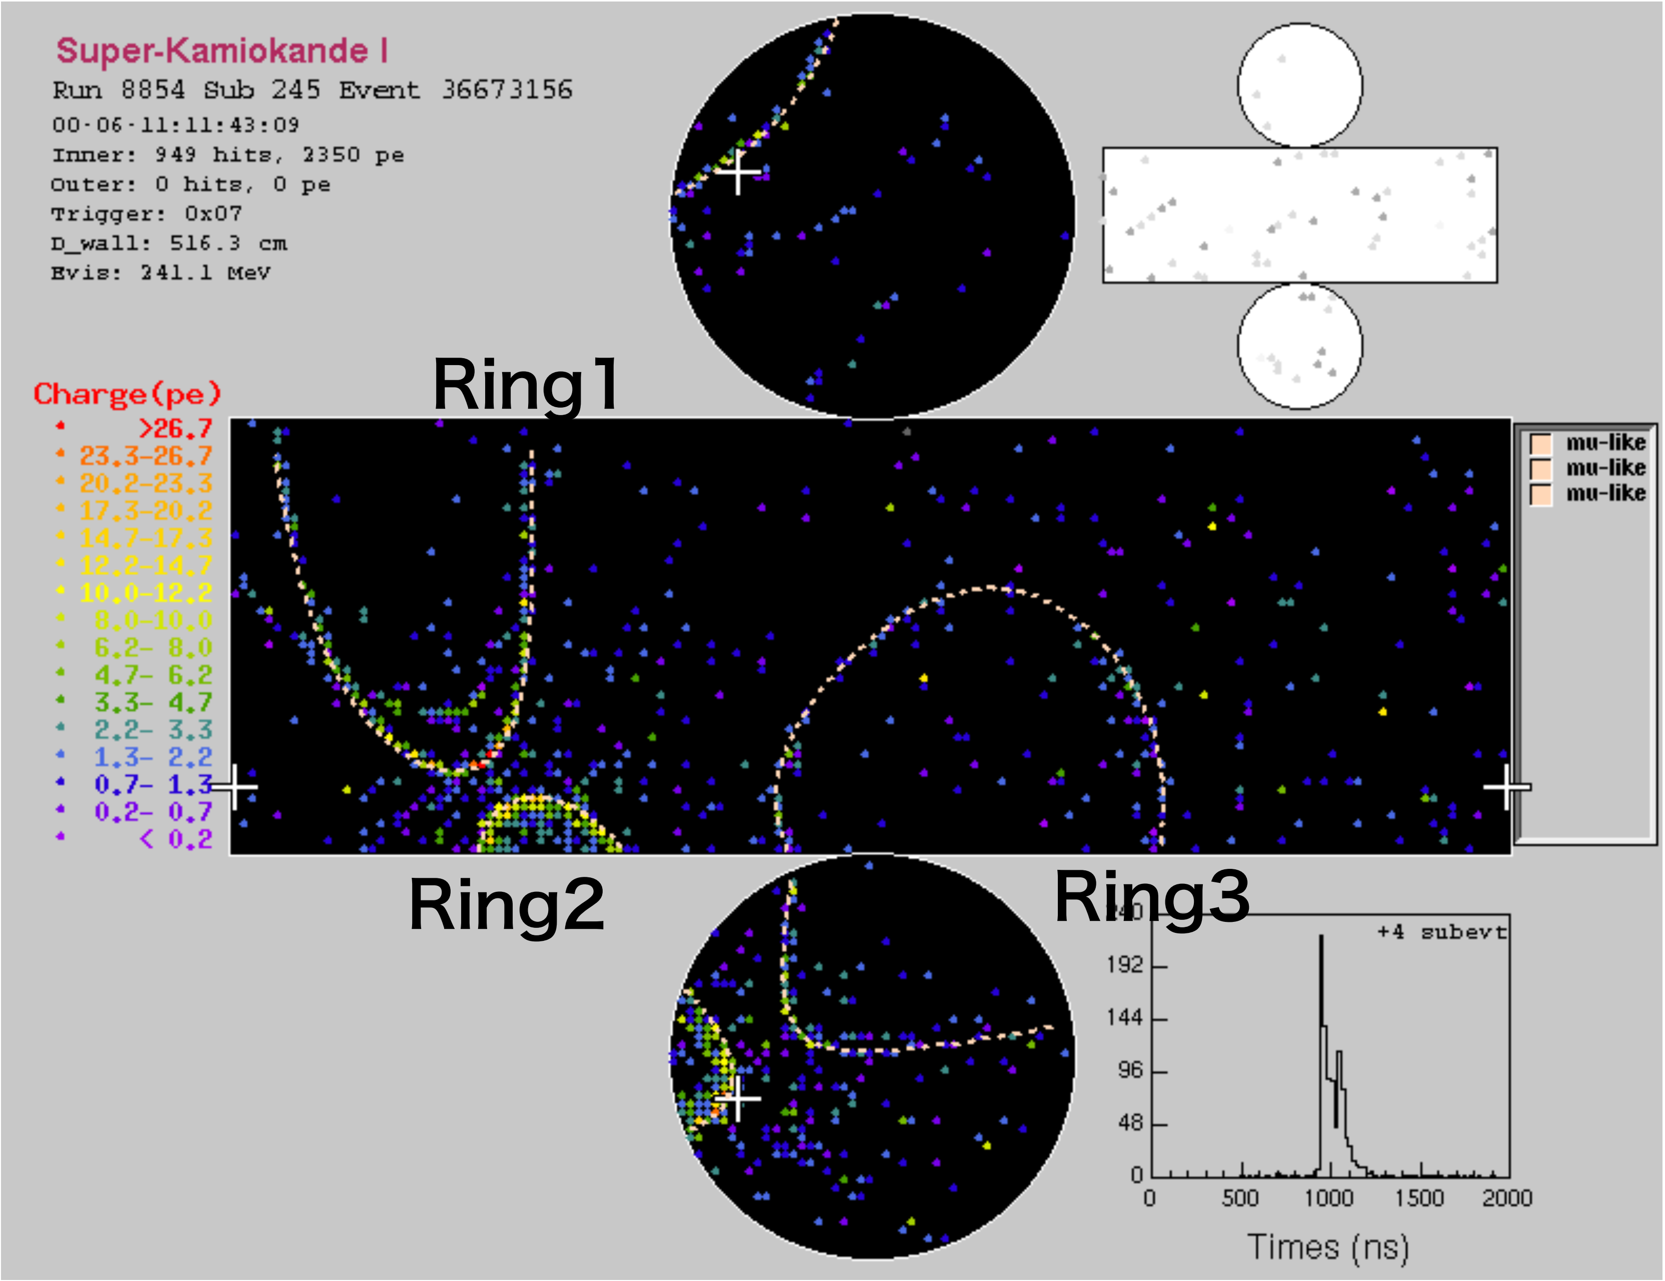


**Ring1**

PID: 2.21 → $\mu$-like

Opening angle → 37.1 deg.

Momentum → 277.0 MeV/c

(expected opening angle → 36.6 deg.)

**Ring2**

PID: 2.55→ $\mu$-like

Opening angle → 36.8 deg.

Momentum → 289.7 MeV/c

(expected opening angle → 37.0 deg.)

**Ring3**

PID: 1.88→ $\mu$-like

Opening angle → 33.8 deg.

Momentum → 223.8 MeV/c

(expected opening angle → 33.9 deg.)

# Typical atmospheric neutrino background MC events



## Note

- Similar events to candidates are also seen in typical background events. (Event displays in p5, 6)

# Typical atmospheric neutrino background MC events ($p \to e^+ \mu^+ \mu^-$)

**True**

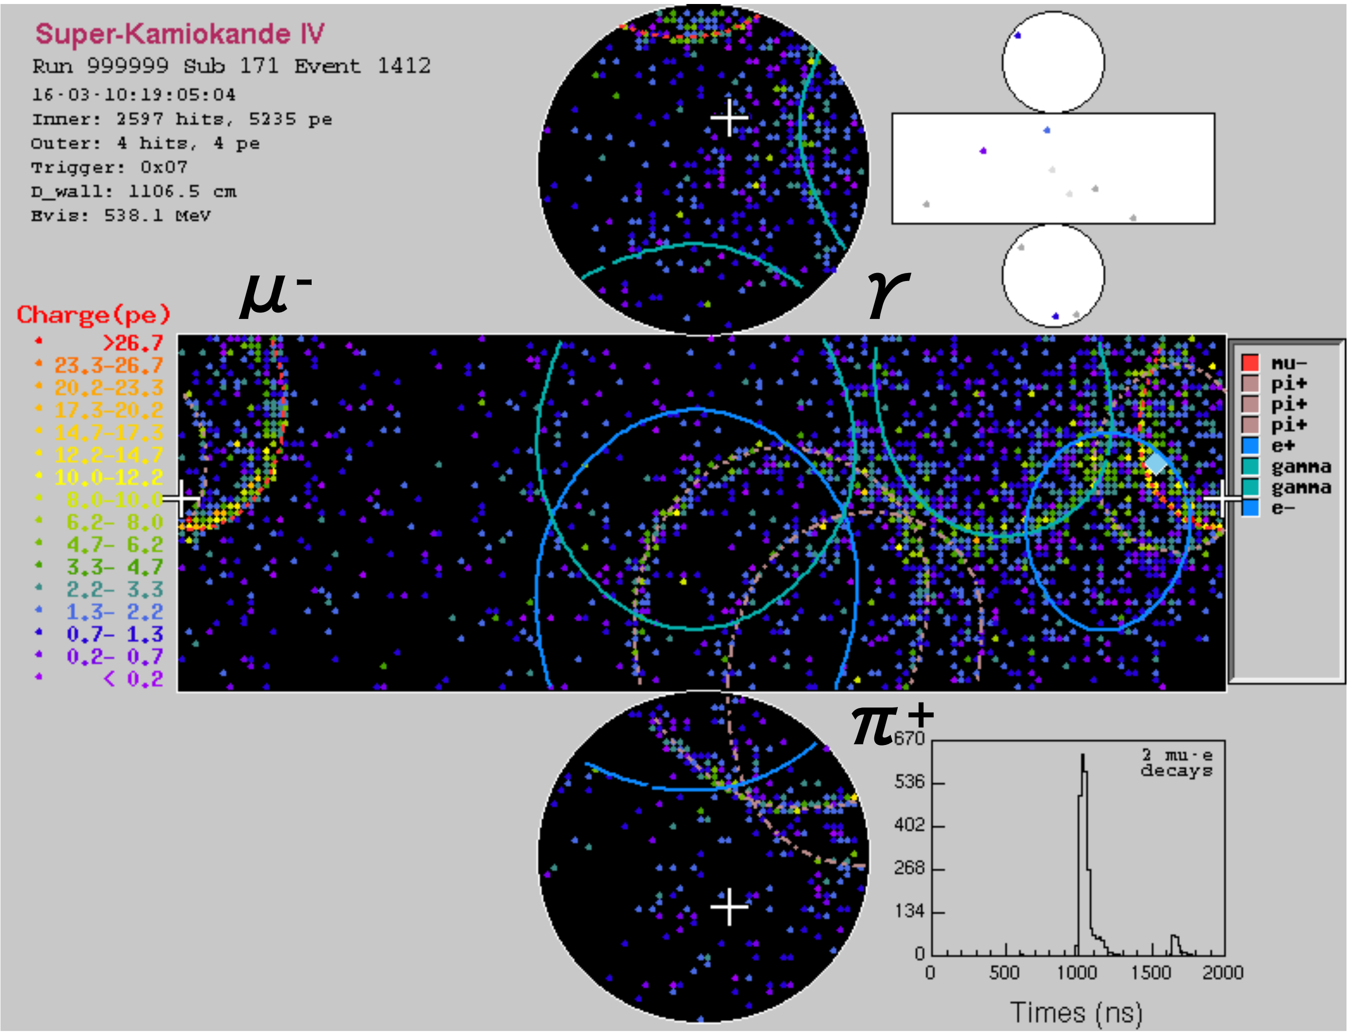


**Reconstructed**

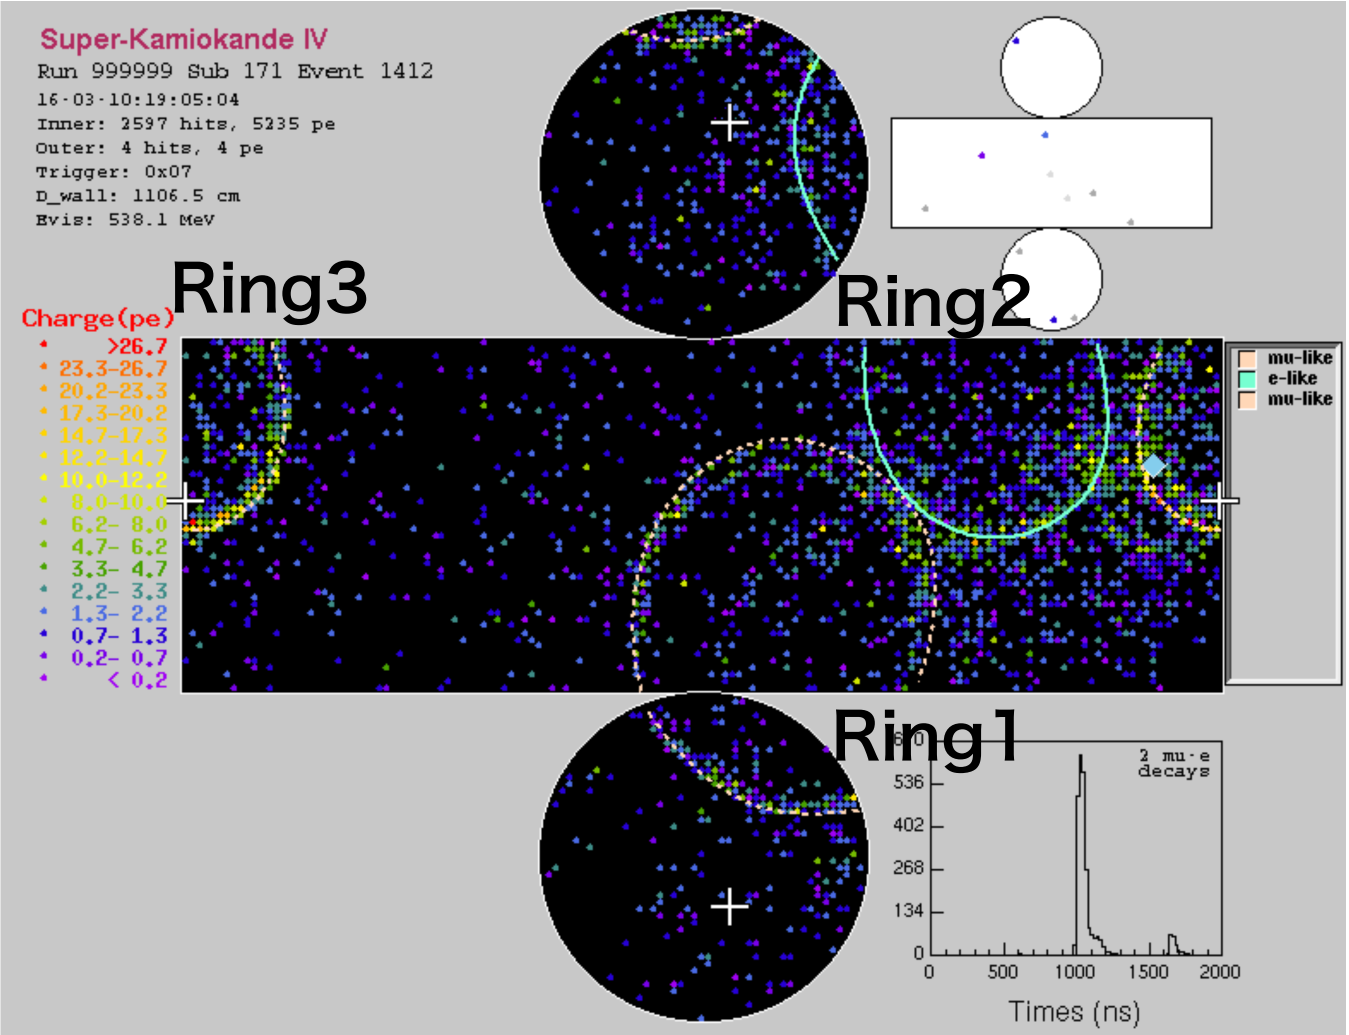


**CC multi $\pi$ ($\nu_\mu p \to \mu^- p \pi^+ \pi^0$)**

# Typical atmospheric neutrino background MC events ($p \to \mu^+\mu^+\mu^-$)



**True** | **Reconstructed**

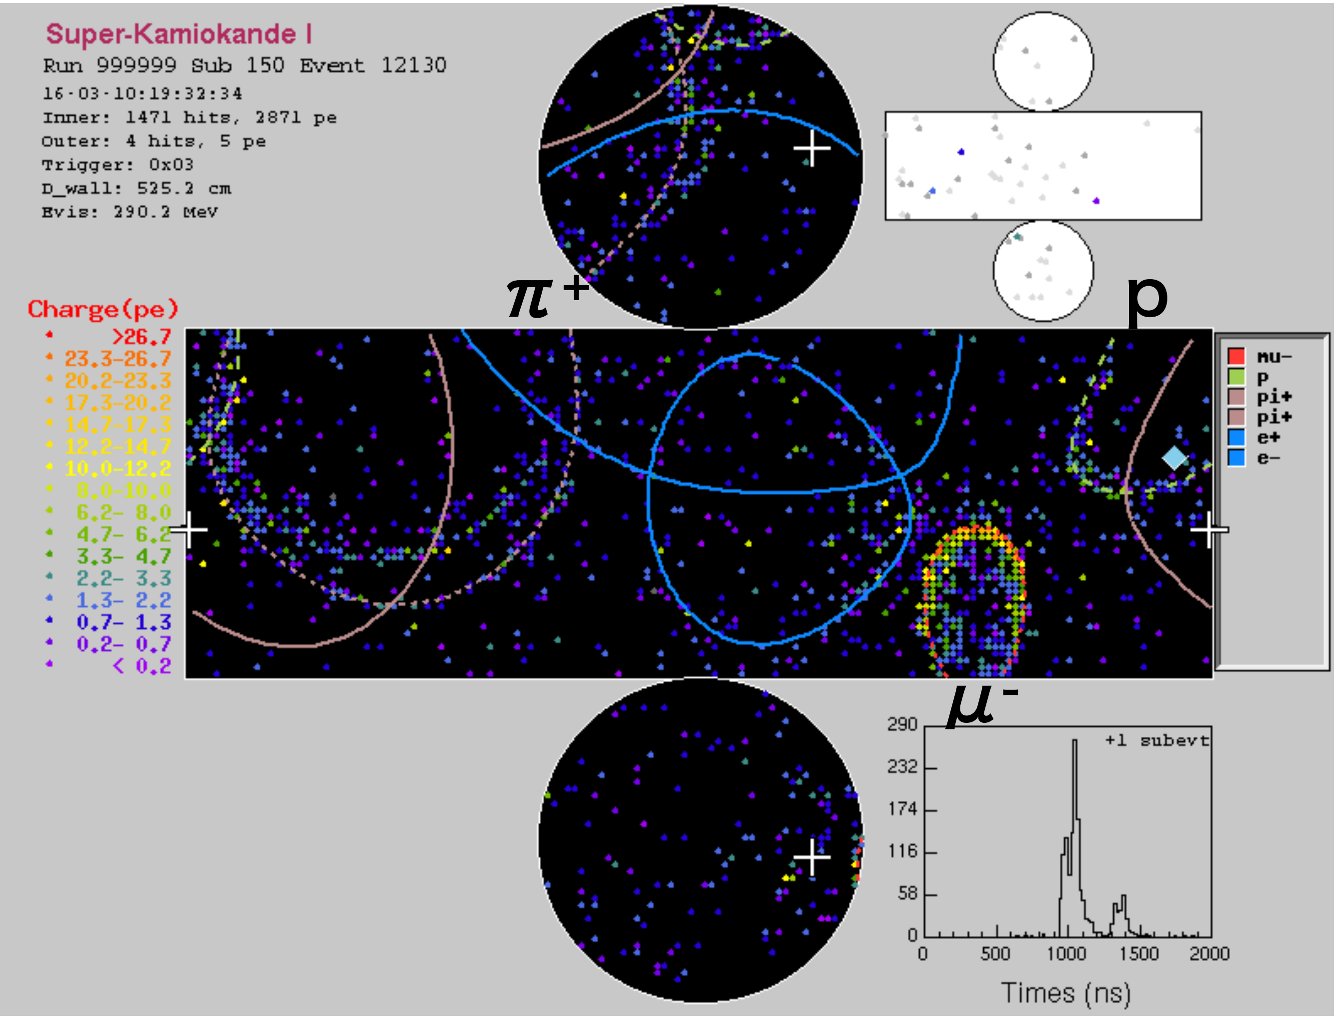


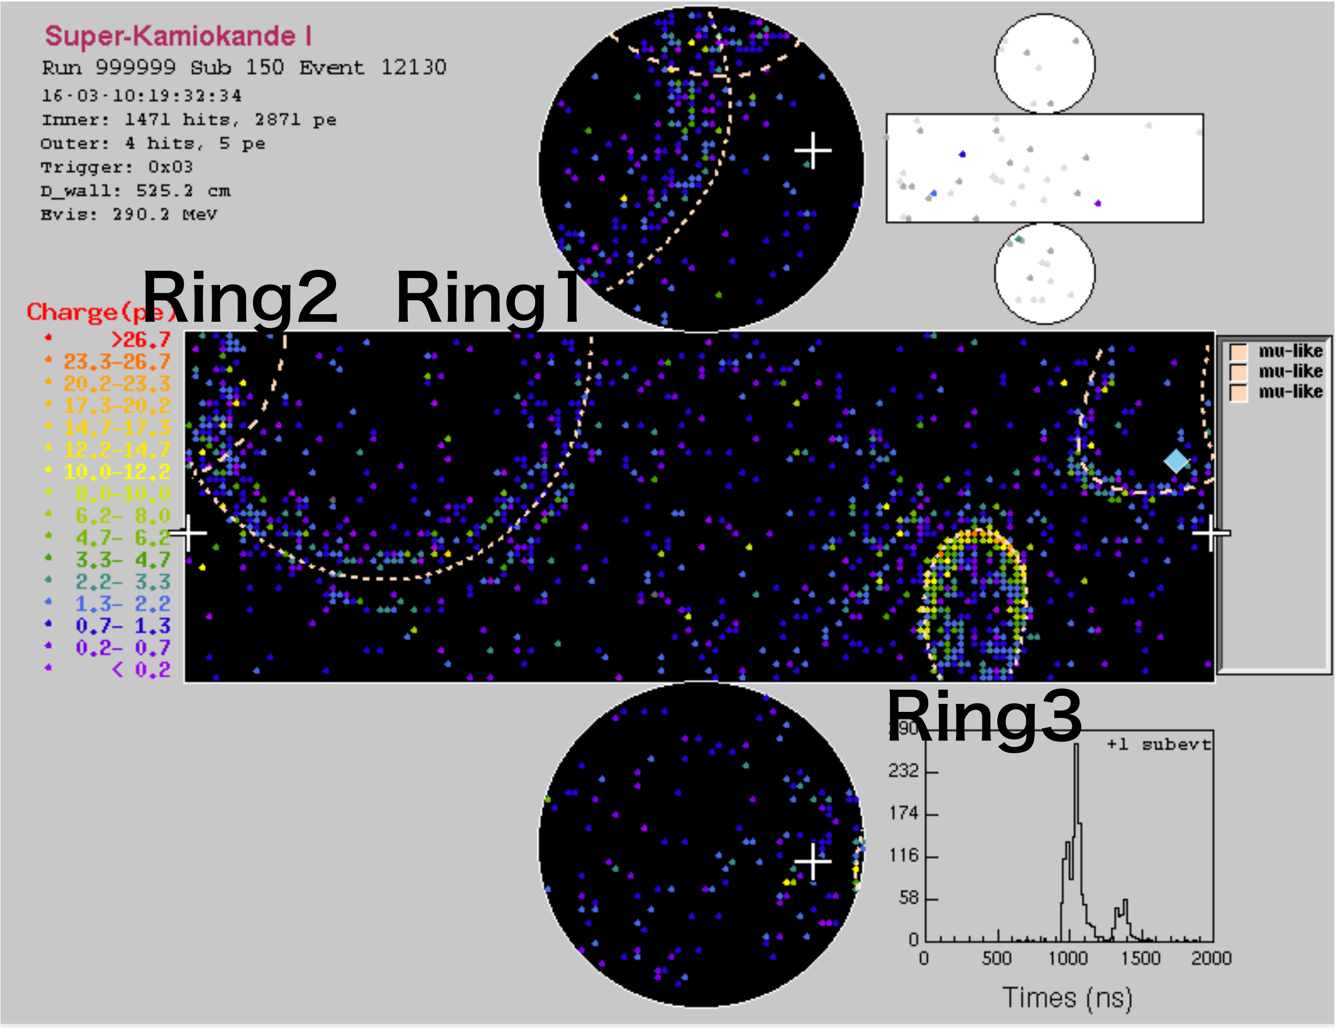


**CC single $\pi$ ($\nu_\mu n \to \mu^- p\ \pi^+$)**
